# Supplementary material for: Navigating the Mirage: A Dual-Path Agentic Framework for Robust Misleading Chart Question Answering
Source: arXiv:2603.28583 source file (2026-07-14)
Supplement: Supplementary file 1 [file appendix.tex]

\setcounter{page}{1}
\section{Supplementary Material}

\subsection{Detailed Dataset Descriptions}
\label{sec:appendix_datasets}

\textbf{Misleading ChartQA.} This large-scale dataset provides a comprehensive testbed for multimodal reasoning under deceptive conditions \citeapp{chen2025unmasking}. 
The test set evaluates the model's structural defense mechanism across 21 distinct categories of visual misleaders and 10 chart types. 
It provides rich multimodal contexts, including standardized chart code, CSV data, and expert explanations, which are critical for testing fine-grained investigative reasoning.

\noindent\textbf{Curated Deceptive Chart Collection.} To enhance the ecological validity of our evaluation and ensure a comprehensive benchmark, we curated a consolidated dataset by aggregating open-source instances from prominent HCI longitudinal studies and literacy assessments. 
Following the evaluation protocols established in recent literature \citeapp{tonglet2025protecting}, we merged multiple sources to mitigate the limited sample sizes inherent in individual datasets, thereby creating a more diverse and statistically robust evaluation suite. 
Specifically, this 110-sample collection draws from CALVI \citeapp{ge2023calvi}, the Lauer \& O'Brien dataset \citeapp{lauer2020deceptive}, and other recent deceptive visualization benchmarks \citeapp{lo2022misinformed, tonglet2025protecting}, focusing on real-world misleading charts tailored to evaluate the framework's ability to resolve epistemic conflicts between visual presentation and underlying data.

\noindent\textbf{Mixed Standard and Misleading Benchmark.} This custom benchmark is designed to monitor the trade-off between adversarial robustness and standard utility. 
The 244 samples are explicitly balanced:
1) For the misleading subset, we sample exactly two instances per fine-grained category (spanning combinations of misleaders and chart types) from the Misleading ChartQA test set, totaling 122 charts.
2) For the standard subset, we sample 122 instances sourced from ChartInsights \citeapp{wu2024chartinsights}. 
We employ a round-robin sampling strategy across seven chart type and question type combinations, yielding roughly 16 to 18 instances per chart type. 
These subsets are combined and randomly shuffled during evaluation.

\subsection{Formal Metric Definitions}
\label{sec:appendix_metrics}

We formally define the three evaluation metrics utilized to dissect the model's performance and error modalities:

\textbf{Accuracy (Acc):} Evaluates the overall effectiveness of the framework. 
It represents the strict percentage of samples where the model successfully predicts the ground-truth correct option $a^*$, overcoming any visual illusions present in the chart.

\textbf{WM (Wrong due to Misleader):} This metric acts as a vulnerability indicator. 
It explicitly quantifies the samples where the model's error is directly attributable to the specific manipulation function $f_{deceptive}$. 
A prediction is counted as WM if the model's output perfectly aligns with the pre-defined ``trap answer'' $a_{trap}$ driven by the misleading visual heuristic.

\textbf{WO (Wrong due to Other factors):} This metric captures benign errors. 
It counts cases where the model fails, but the predicted answer aligns with neither the ground-truth $a^*$ nor the deceptive lure $a_{trap}$. 
Such errors typically indicate deficiencies in basic chart reading, hallucination, or formatting failures, rather than a successful cognitive hijacking by the chart designer.

\subsection{Robustness to OCR Backbones}
To assess the sensitivity of our framework to the choice of the underlying OCR engine, we conducted an additional robustness study by replacing the default OCR backbone (\textit{LlamaParser}) with two widely-used open-source and industrial alternatives: \textbf{DeepSeek-OCR v2}\citeapp{wei2026deepseek} and \textbf{Paddle OCR (PP-StructureV3)}\citeapp{cui2025paddleocr30technicalreport}.

As shown in Table \ref{tab:ocr_robustness}, the performance remains remarkably consistent across different backbones. While LlamaParser (integrated within the Full ChartCynics train-free pipeline) achieves an accuracy of 60.66\%, switching to DeepSeek-OCR v2 and Paddle OCR yields accuracies of 58.36\% and 58.03\%, respectively.

Interestingly, while the WM (Wrong due to Misleader) rate varies slightly, with DeepSeek-OCR v2 demonstrating a slightly lower vulnerability (21.64\%) compared to Paddle OCR (25.57\%), the overall trend confirms that the core defensive capability of our framework is derived from the structural reasoning and cross-modal verification rather than the specific OCR implementation. This suggests that as long as the OCR can faithfully reconstruct the underlying data table (CSV), our framework can effectively mitigate visual deceptive heuristics.

\begin{table}[h]
\centering
\caption{Impact of Different OCR Backbones on the Full Pipeline (Train-free Setting).}
\label{tab:ocr_robustness}
\begin{tabular}{lccc}
\toprule
\textbf{OCR Backbone} & \textbf{Acc $\uparrow$} & \textbf{WM $\downarrow$} & \textbf{WO $\downarrow$} \\ \midrule
LlamaParser (Default) & \textbf{60.66} & 24.26 & \textbf{15.08} \\
DeepSeek-OCR v2       & 58.36 & \textbf{21.64} & 20.00 \\
Paddle OCR (PP-StructureV3) & 58.03 & 25.57 & 16.40 \\
\bottomrule
\end{tabular}
\end{table}

\subsection{Token Consumption and Resource Analysis}

To evaluate the computational footprint of the ChartCynics framework, we benchmarked the token consumption across each modular component. This analysis provides insight into the resource overhead associated with our dual-path design. Table \ref{tab:token_consumption} details the average number of prompt, completion, and total tokens required for different stages of the pipeline.

\begin{itemize}
    \item \textbf{Vision Path ($\mathcal{P}_v$):} This path accounts for the visual investigation tokens. The \textbf{VLM Path} (holistic) maintains a relatively light footprint, whereas the \textbf{Crop-VLM Path} (investigative) requires significantly higher prompt tokens. This increase is primarily due to the inclusion of high-resolution visual tokens and the detailed prompts necessary for localized analysis.
    \item \textbf{Data Path Stage ($\mathcal{P}_d$):} The \textbf{OCR Reasoning} component remains the most resource-efficient stage. By establishing a ``literal backbone'' with minimal token overhead, it allows the framework to anchor visual heuristics in numerical truth without exhausting the context window.
    \item \textbf{Summarizer Joint Inference ($\mathcal{S}$):} These stages represent the \textbf{Detective Chain-of-Thought (D-CoT)} fusion. The \textbf{Crop Summary} carries the largest cumulative token load, as it integrates the dense \textbf{ROI-based investigation} results to resolve complex epistemic conflicts between visual and numerical data.
\end{itemize}

\textbf{Resource Distribution Analysis:} The results indicate that the \textbf{Crop-augmented VLM Diagnostic} ($f_{diag}$) is the most resource-intensive module, consuming over 14,000 tokens per call. This high consumption is attributed to the multi-scale visual sampling and the exhaustive investigative prompts required to unmask sophisticated visual traps. Despite this expenditure, the total token consumption is justified by the framework’s significant gains in adversarial robustness through rigorous cross-modal verification.

\begin{table}[h]
\centering
\caption{Average Token Consumption per Module.}
\label{tab:token_consumption}
\begin{tabular}{llccc}
\toprule
\textbf{Category} & \textbf{Sub-module} & \textbf{Prompt} & \textbf{Comp.} & \textbf{Total} \\
\midrule
\textbf{VLM Path} & VLM Diagnostic ($f_{diag}$) & 2,326 & 137 & 2,463 \\
& VLM Reasoning ($f_{reason}$) & 2,486 & 254 & 2,740 \\
\midrule
\textbf{Crop-VLM Path} & Crop-VLM Diagnostic ($f_{diag}$) & 13,897 & 447 & 14,344 \\
& Crop-VLM Reasoning ($f_{reason}$) & 2,427 & 608 & 3,035 \\
\midrule
\textbf{OCR Stage ($\mathcal{P}_d$)} & OCR Reasoning & 908 & 301 & 1,209 \\
\midrule
\textbf{Global Summary ($\mathcal{S}$)} & VLM Diagnostic ($f_{diag}$) & 2,325 & 118 & 2,443 \\
& Summarizer Reasoning ($\mathcal{S}$) & 3,963 & 539 & 4,502 \\
\midrule
\textbf{Crop Summary ($\mathcal{S}$)} & Crop-VLM Diagnostic ($f_{diag}$) & 14,725 & 484 & 15,209 \\
& Summarizer Reasoning ($\mathcal{S}$) & 3,941 & 453 & 4,394 \\
\bottomrule
\end{tabular}
\end{table}

\subsection{Multimedia Materials and Open-Source Release}
\label{sec:appendix_multimedia_code}

To facilitate an intuitive understanding of the ChartCynics framework and the challenges posed by Misleading ChartQA, we provide \textbf{multimedia supplementary material} together with a \textbf{public code release}.

\paragraph{Video demonstration.}
We include a supplementary video (submitted as \texttt{ChartCynics\_Demo.mp4}), structured into two segments: \emph{(1)~Methodology and Problem Overview} and \emph{(2)~Real-World Usage Demo}.

\paragraph{Open-source implementation.}
We release our implementation (including inference-time pipelines, distillation, supervised fine-tuning, and evaluation scripts) to support reproducibility and extension. An anonymized snapshot is available at \url{https://anonymous.4open.science/r/ChartCynics-7D52/}.

\newpage

% 请在导言区（\begin{document}之前）加入以下宏包：
% \usepackage{tcolorbox}
% \usepackage{xcolor}

\subsection{Prompt Templates}
\label{sec:appendix_prompts}
In this section, we detail the exact prompt templates used for each modular component in the ChartCynics framework. System prompts are denoted in \textit{italics}, and variables populated at runtime are enclosed in braces (e.g., \texttt{\{question\}}).

\subsubsection{VLM Path}
This sub-section outlines the prompts used for the isolated two-agent vision stack.

\begin{tcolorbox}[colback=blue!5,colframe=blue!70,title=\textbf{Prompt: VLM Diagnostic ($f_{diag}$)}]
\textit{\textbf{System Prompt:} You are a data visualization review expert who identifies misleading designs in charts.}

\vspace{2mm}
\textbf{User Prompt:} \\
You are a meticulous data visualization review expert. Your sole task is to inspect the given chart for any misleading design elements.

\textbf{\#\#\# Your Task:}
\begin{enumerate}
    \item \textbf{Analyze the Chart}: Scrutinize the chart for common misleading techniques:
    \begin{itemize}
        \item \textbf{Axis Manipulation}: Does the Y-axis start at 0? Is the scale linear and appropriate?
        \item \textbf{Improper Order}: Is the X-axis or legend ordered logically (e.g., chronologically)?
        \item \textbf{Visual Distortion}: Do visual elements (e.g., 3D effects, area sizes) accurately represent the data proportions?
        \item \textbf{Data Cherry-Picking}: Are there signs that the data has been selectively presented?
    \end{itemize}
    \item \textbf{Output a Diagnostic Report}:
    \begin{itemize}
        \item \textbf{Do not answer any questions about the chart's content.}
        \item Your output must be a brief, precise diagnostic report that clearly identifies the misleading design.
        \item Crucially, the report must conclude with a clear "Action Directive" that instructs how to avoid the trap and interpret the data correctly.
    \end{itemize}
\end{enumerate}

\textbf{\#\#\# Example Output Format:} \\
Diagnosis: The chart's X-axis is in reverse chronological order (from Dec to Jan), which creates a false visual impression of a decline. \\
Action Directive: To determine the true trend, the visual line slope must be ignored. Instead, read the data points strictly from right to left.

Now, analyze the provided chart and output your diagnostic report and action directive.
\end{tcolorbox}

\begin{tcolorbox}[colback=purple!5,colframe=purple!70,title=\textbf{Prompt: VLM Reasoning ($f_{reason}$)}]
\textit{\textbf{System Prompt:} You are an AI analyst who strictly follows expert instructions to analyze charts and answer questions.}

\vspace{2mm}
\textbf{User Prompt:} \\
You are a logically rigorous AI analyst. You have received an expert's "Diagnostic Report" containing a critical warning on how to correctly interpret the chart. Your primary principle is: \textbf{You must unconditionally trust and follow the report's directives.}

\textbf{\#\#\# Expert Diagnostic Report:} \\
\texttt{\{diagnosis\_report\}}

\textbf{\#\#\# Question:} \\
\texttt{\{question\}}

\textbf{\#\#\# Options:} \\
\texttt{\{formatted\_options\}}

\textbf{\#\#\# Your Instructions:}
\begin{enumerate}
    \item \textbf{Adopt the Directive}: All of your reasoning must be based on the "Action Directive" from the expert report. Do not rely on your first visual impression.
    \item \textbf{Plan Your Steps}: In your explanation, first state how you will adjust your analysis strategy based on the directive. For example: "As instructed, I will ignore the chart's downward curve and instead read the data from right to left..."
    \item \textbf{Execute and Answer}: Strictly follow your new strategy to derive a conclusion and select the correct option.
\end{enumerate}

\textbf{\#\#\# Output Format:}
\begin{itemize}
    \item \textbf{First Line}: Must be the single letter of your chosen option (A, B, C, or D).
    \item \textbf{Subsequent Lines}: Provide a detailed explanation that clearly shows how you used the "Diagnostic Report" to arrive at your answer.
\end{itemize}
Now, answer the question with careful consideration of all the information provided.
\end{tcolorbox}

\subsubsection{Crop-VLM Path}
This sub-section outlines the prompts used for the crop-augmented isolated vision stack. Note that the \textit{Crop-VLM Reasoning ($f_{reason}$)} module shares the exact same prompt template as the \textit{VLM Reasoning ($f_{reason}$)} module shown above, differing only in that the input \texttt{\{diagnosis\_report\}} is richer as it is derived from multi-turn crop diagnostics.

\begin{tcolorbox}[colback=cyan!5,colframe=cyan!60!black,title=\textbf{Prompt: Crop-VLM Diagnostic ($f_{diag}$)}]
\textit{\textbf{System Prompt:} You are a data visualization review expert who identifies misleading designs in charts.}

\vspace{2mm}
\textbf{Turn 1 (User - Full Image):} \\
Here is the full chart. Please observe it carefully before I provide you with detail crops of specific components. \textit{[Attached: Full Image]}

\textbf{Turn 2 (User - Title Crop):} \\
This is a close-up of the chart title. In one sentence, describe what you observe: is the title consistent with what the chart shows, or does it appear exaggerated or misleading? \textit{[Attached: Title Crop]}

\textbf{Turn 3 (User - Legend Crop):} \\
This is a close-up of the chart legend. In one sentence, describe what you observe: does the legend order match the visual order of elements, and are all categories present and correctly labeled? \textit{[Attached: Legend Crop]}

\textbf{Turn 4 (User - X-Axis Crop):} \\
This is a close-up of the X-axis. In one sentence, describe what you observe: is the order logical (e.g., chronological), and are there any missing, reversed, or unevenly spaced labels? \textit{[Attached: X-Axis Crop]}

\textbf{Turn 5 (User - Y-Axis Crop):} \\
This is a close-up of the Y-axis. In one sentence, describe what you observe: does the axis start at 0, is the scale linear and consistent, and is there any truncation or irregular interval? \textit{[Attached: Y-Axis Crop]}

\textbf{Turn 6 (User - Final Conclusion):} \\
Based on the full chart and all the component crops you have analyzed above, now output your final diagnostic report.

\textbf{\#\#\# Example Output Format:} \\
Diagnosis: The chart's X-axis is in reverse chronological order (from Dec to Jan), which creates a false visual impression of a decline. \\
Action Directive: To determine the true trend, the visual line slope must be ignored. Instead, read the data points strictly from right to left.

Do not answer any question about the chart content. Only output the diagnostic report and action directive.
\end{tcolorbox}

\subsubsection{OCR Stage}
The OCR Reasoning module directly takes the serialized Markdown table and performs multiple-choice question answering.

\begin{tcolorbox}[colback=gray!5,colframe=black!70,title=\textbf{Prompt: OCR Reasoning}]
\textit{\textbf{System Prompt:} You are a helpful AI assistant designed for analyzing chart data and answering multiple-choice questions and give explanations.}

\vspace{2mm}
\textbf{User Prompt:} \\
You are given chart information in markdown format and a multiple-choice question related to it.

\textbf{\#\#\# Chart Information (Markdown):} \\
\texttt{\{markdown\_text\}}

\textbf{\#\#\# Question:} \\
\texttt{\{question\}}

\textbf{\#\#\# Options:} \\
\texttt{\{formatted\_options\}}

\textbf{\#\#\# Instructions:}
\begin{itemize}
    \item \textbf{Only output the selected option on the first line (A, B, C, or D).}
    \item Then, on a new line, \textbf{provide a detailed explanation} on why this choice is correct based on the chart information.
    \item Your response \textbf{must always start with a single letter (A, B, C, or D)}.
\end{itemize}
Now, answer accordingly.
\end{tcolorbox}

\newpage

\subsubsection{Global Summary \& Crop Summary ($\mathcal{S}$)}
The final Agentic Fusion modules (Summarizer Reasoning) resolve conflicts between visual heuristics (via the Diagnostic Report from either VLM or Crop-VLM) and literal data (via OCR Markdown) through a formal Detective Chain-of-Thought (D-CoT). Note that the \textit{VLM Diagnostic} and \textit{Crop-VLM Diagnostic} components in these stages use the identical prompts to those presented in the Path sections above.

\begin{tcolorbox}[colback=green!5,colframe=green!60!black,title=\textbf{Prompt: Summarizer Reasoning ($\mathcal{S}$)}]
\textit{\textbf{System Prompt:} You are an AI analyst who strictly follows expert instructions to analyze charts and answer questions. Output the option letter (A/B/C/D) on the first line, then your explanation.}

\vspace{2mm}
\textbf{User Prompt:} \\
\textbf{\#\#\# Role \& Directive} \\
You are an expert Data Analysis Detective evaluating a chart flagged as "highly misleading." \\
\textbf{GOLDEN RULES OF EVIDENCE}:
\begin{enumerate}
    \item \textbf{Defy Visual Intuition}: Never trust your first visual impression (e.g., the apparent height of bars, the steepness of a line).
    \item \textbf{Dynamic OCR Trust}:
    \begin{itemize}
        \item \textbf{High Trust}: If the chart contains \textit{explicit numerical or textual labels} plotted on or near the data points, trust the \texttt{OCR Data} completely over the visual scale.
        \item \textbf{Low Trust / Skepticism}: If the chart lacks explicit data labels, or if visual elements extend beyond the display area (\texttt{Exceeding the Canvas}), do NOT blindly trust the OCR numbers. In these cases, OCR might be an imprecise estimation or hallucination. You must rely more heavily on the \texttt{Diagnostic Report}'s logical deduction.
    \end{itemize}
    \item \textbf{The "Incomplete Period" Trap}: Always scrutinize the final data point on a time axis. Be highly alert to whether the last period (e.g., the current year or month) is actually complete, or if it is an ongoing, partial period deceptively plotted next to full periods.
\end{enumerate}

\textbf{\#\#\# Misleading Taxonomy (Reference Guide)} \\
When determining how the chart deceives the viewer, you must classify the deception using one or more of the following formal taxonomies:
\textit{[Detailed 4-category taxonomy rules (e.g., Manipulated Annotation, Data, Scale, Visual Encoding) provided here...]}

\textbf{\#\#\# Input Data}
\begin{itemize}
    \item \textbf{OCR Data}: \texttt{\{ocr\_markdown\}}
    \item \textbf{Diagnostic Report}: \texttt{\{diagnosis\_report\}}
    \item \textbf{Question}: \texttt{\{question\}}
    \item \textbf{Options}: \texttt{\{formatted\_options\}}
\end{itemize}

\textbf{\#\#\# Investigative Chain-of-Thought} \\
Please execute the following detective reasoning steps strictly in order, documenting your thought process inside the \texttt{<Thinking>} tags:
\begin{enumerate}
    \item \textbf{Read \& Anchor}: Carefully read the "Action Directive" in the \texttt{Diagnostic Report}. Identify exactly which area of the chart or which visual feature the report warns you to be highly skeptical of.
    \item \textbf{Evidence Gathering \& Verification}: Extract the relevant numbers from the \texttt{OCR Data}.
    \begin{itemize}
        \item \textit{Trust Check}: State explicitly whether these OCR values come from clear, explicit labels on the chart OR if they are derived from unlabelled/out-of-bounds visual elements (which requires skepticism).
        \item \textit{Temporal Check}: Examine the time axis. Is the most recent data point representing a complete period, or is it an incomplete period masquerading as a full one?
    \end{itemize}
    \item \textbf{Misleading Identification}: Synthesize the report's warnings, the verified OCR data, and your visual cross-checks. You MUST categorize the chart's deception using one or more specific classes from the \texttt{Misleading Taxonomy} provided above. Explain the exact illusion created.
    \item \textbf{Sufficiency Check}: \textbf{[CRITICAL STEP]} Given the OCR trust level and the diagnostic warnings, do you have enough reliable evidence to answer the question? If the OCR is deemed unreliable due to missing labels/exceeding canvas, or if the time period is deceptively incomplete, strongly consider if the question "Cannot be inferred" or has "Inadequate information."
    \item \textbf{Option Evaluation}: Based \textit{only} on the reality-checked data (or the conclusion from Step 4 that evidence is insufficient), evaluate every Option. Point out the trap answers designed for those who fell for the visual illusion, and lock in the final correct answer.
\end{enumerate}

\textbf{\#\#\# Output Format:}
\begin{itemize}
    \item \textbf{The first line MUST be a single option letter (A/B/C/D), and nothing else.}
    \item From the second line, provide your explanation, which should reflect the two-step process.
\end{itemize}
\end{tcolorbox}

\newpage
\subsubsection{Data Distillation (SFT Golden Chain)}
\label{sec:appendix_distill}
This sub-section specifies the \textbf{teacher-only} prompt used to synthesize golden chain-of-thought supervision for supervised fine-tuning. The teacher receives \textit{privileged oracle fields} (ground-truth answer, trap answer, CSV, explanation) and must emit a student-imitable trace that appears to be derived only from the chart image and the \textit{visible} modalities (OCR markdown and diagnostic report). At runtime, the multimodal user message includes the chart image plus the text below.

\begin{tcolorbox}[colback=orange!5,colframe=orange!80!black,title=\textbf{Prompt: Teacher Distillation ($f_{\mathrm{distill}}$)}]
\textit{\textbf{System Prompt:} (none; role is embedded in the user message below, or set to a neutral assistant if your API requires it.)}

\textbf{User Prompt:} \\
You are an Expert Data Analysis Detective training a junior analyst. \\
You are given a misleading chart and its associated data streams. Your task is to write a flawless, step-by-step reasoning chain that exposes the chart's deception.

\textbf{\#\#\# ORACLE KNOWLEDGE (Privileged --- use only to ensure correctness of the chain; the junior must not see this section in deployment):}
\begin{itemize}
    \item \textbf{True Answer:} \texttt{\{correct\_answer\}}
    \item \textbf{Visual Trap Answer:} \texttt{\{wrong\_trap\_answer\}}
    \item \textbf{Misleader Technique:} \texttt{\{misleader\_technique\}}
    \item \textbf{True Data Distribution (CSV):} \\
    \texttt{\{csv\_text\}}
    \item \textbf{Expert Explanation:} \texttt{\{expert\_explanation\}}
\end{itemize}

\textbf{\#\#\# VISIBLE INPUTS (What the junior analyst can see at test time):}
\begin{itemize}
    \item \textbf{OCR Markdown:} \texttt{\{ocr\_markdown\}}
    \item \textbf{Diagnostic Report:} \texttt{\{diagnosis\_report\}}
    \item \textbf{Question:} \texttt{\{question\}}
    \item \textbf{Options:} \texttt{\{formatted\_options\}}
\end{itemize}

\textbf{\#\#\# INSTRUCTION:} \\
Reverse-engineer the thought process. Using the ORACLE KNOWLEDGE to guarantee accuracy, write the reasoning chain \textbf{as if} you were deducing it purely from the VISIBLE INPUTS and the chart image. \\
You \textbf{MUST} output \textbf{strictly} in the following four-stage XML format, with \textbf{no} text before or after the XML blocks.

\textbf{Required structure:}
\begin{verbatim}
<Visual_Heuristic>
...
</Visual_Heuristic>

<OCR_Validation>
...
</OCR_Validation>

<Ambiguity_Resolution>
...
</Ambiguity_Resolution>

<Answer>
...
</Answer>
\end{verbatim}

\textbf{Block semantics:}
\begin{itemize}
    \item \texttt{<Visual\_Heuristic>}: Explain why a careless viewer would choose option \texttt{\{wrong\_trap\_answer\}} from first visual impression.
    \item \texttt{<OCR\_Validation>}: Examine the OCR markdown; extract explicit numerical boundaries, axis scales, or legends, and relate them to the true data distribution.
    \item \texttt{<Ambiguity\_Resolution>}: State the conflict; explicitly identify the case as \texttt{\{misleader\_technique\}} and how the visual impression contradicts OCR and truth.
    \item \texttt{<Answer>}: The final option label only, matching \texttt{\{correct\_answer\}} (e.g., a single letter A/B/C/D as used in the dataset).
\end{itemize}

Now produce the four XML blocks for the provided chart and inputs.
\end{tcolorbox}
